# Supplementary material for: AdaBest: Minimizing Client Drift in Federated Learning via Adaptive Bias Estimation
Source: arXiv:2204.13170 source file (2023-07-24)
Supplement: Supplementary file 1 [file overfitting.pdf]

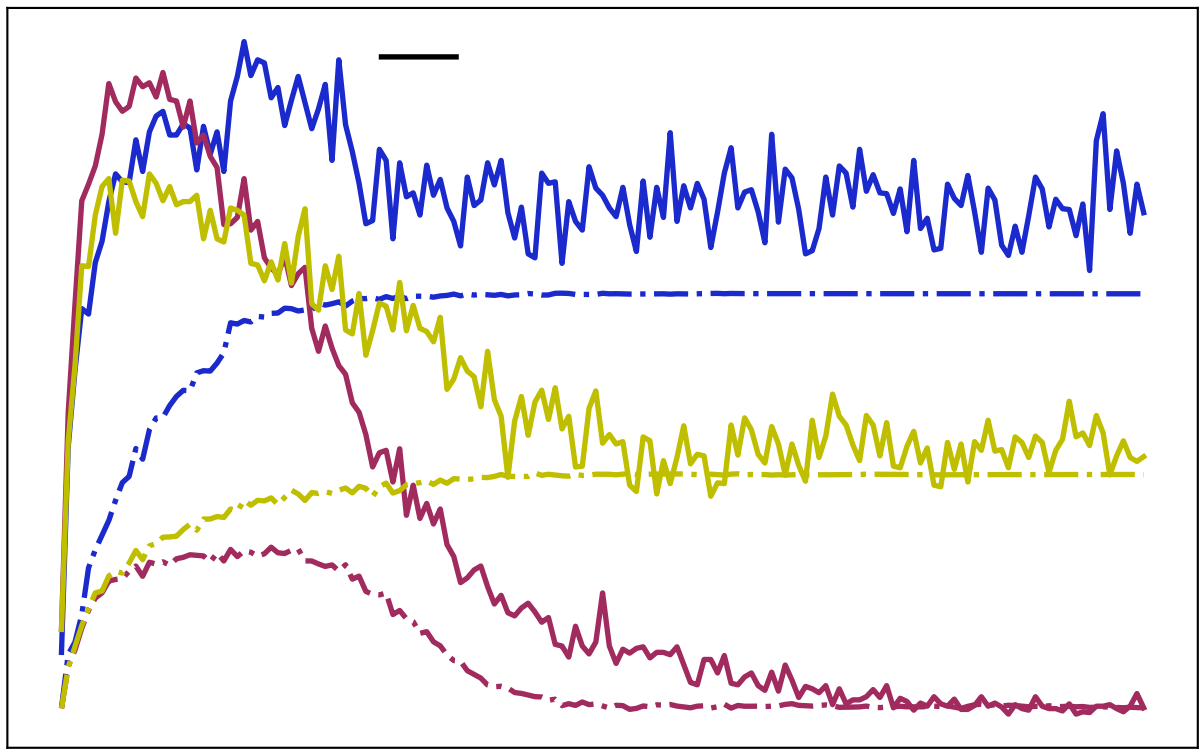

— . —



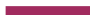

The first part of the document discusses the importance of maintaining accurate records of all transactions and the role of the auditor in ensuring the integrity of the financial statements. It also highlights the need for transparency and accountability in the reporting process.

The second part of the document provides a detailed overview of the audit process, including the planning stage, the execution of the audit, and the final reporting stage. It also discusses the various types of audit opinions that can be issued and the implications of each.

The third part of the document focuses on the ethical considerations that auditors must take into account when performing their duties. It discusses the importance of independence, objectivity, and integrity, and provides guidance on how to handle potential conflicts of interest.

The fourth part of the document discusses the role of the auditor in the broader context of the financial system. It highlights the importance of the auditor in providing assurance to investors and other stakeholders, and discusses the challenges that auditors face in this role.

The fifth part of the document provides a summary of the key points discussed in the document and offers some final thoughts on the importance of the audit process.
