# Supplementary material for: AdaBest: Minimizing Client Drift in Federated Learning via Adaptive Bias Estimation
Source: arXiv:2204.13170 source file (2023-07-24)

1

1

1

1

1

1

















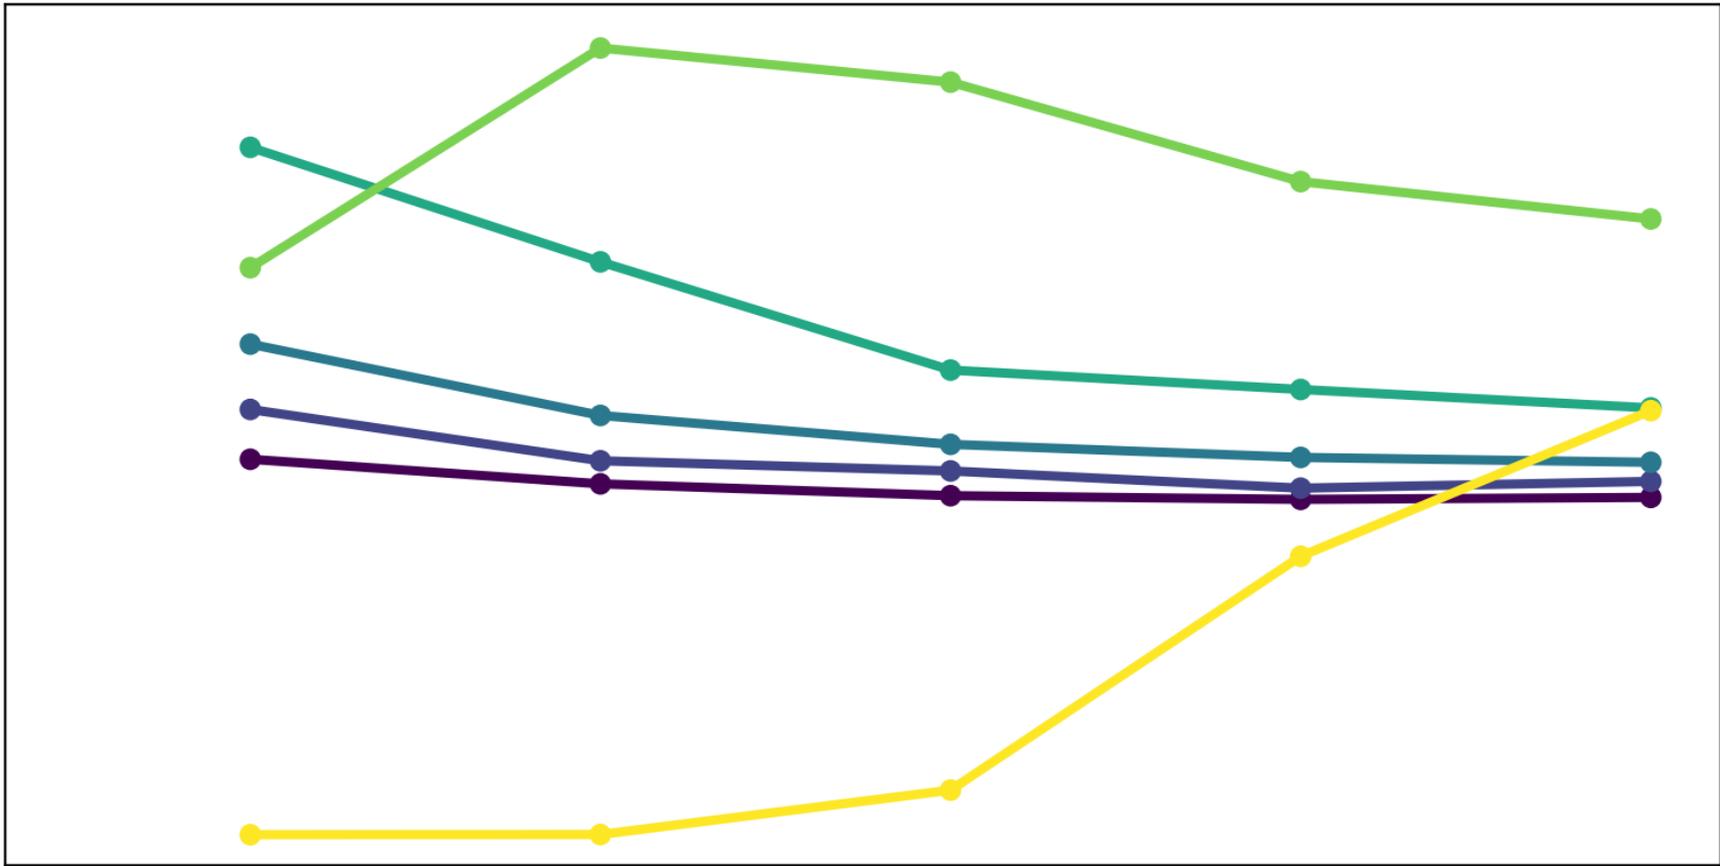

Supplement: Supplementary file 2 [file beta_sensitivity.pdf]
