# Supplementary material for: AdaBest: Minimizing Client Drift in Federated Learning via Adaptive Bias Estimation
Source: arXiv:2204.13170 source file (2023-07-24)
Supplement: Supplementary file 3 [file mu_sensitivity.pdf]

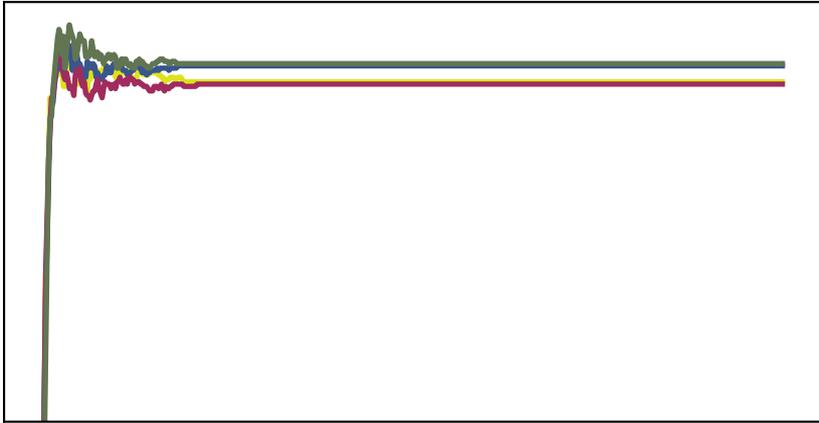





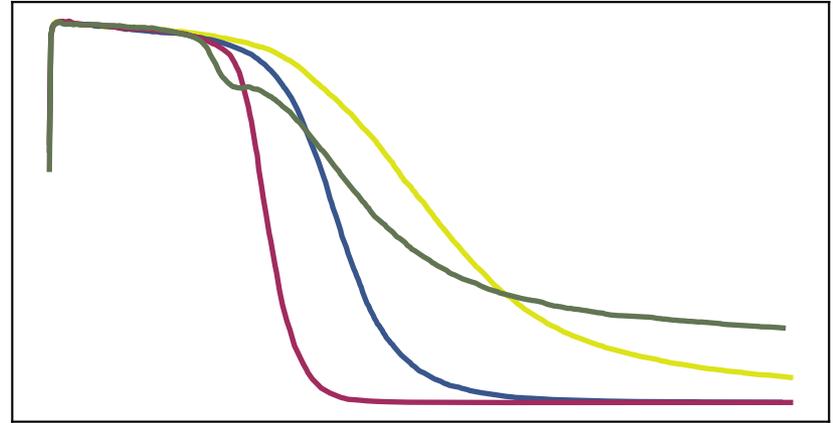





















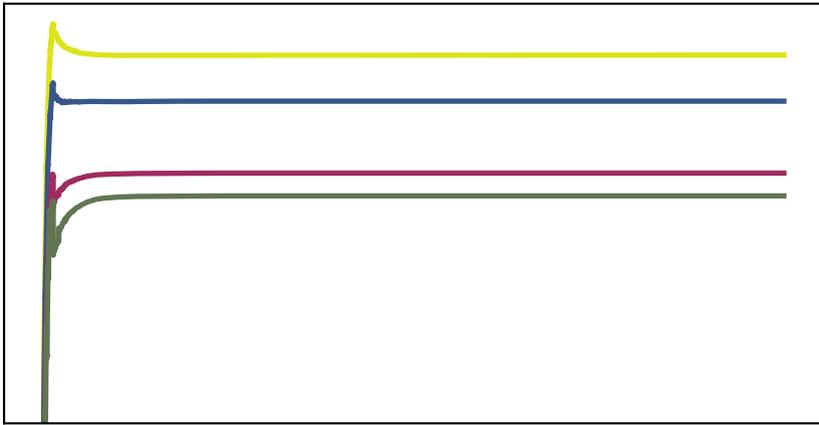

















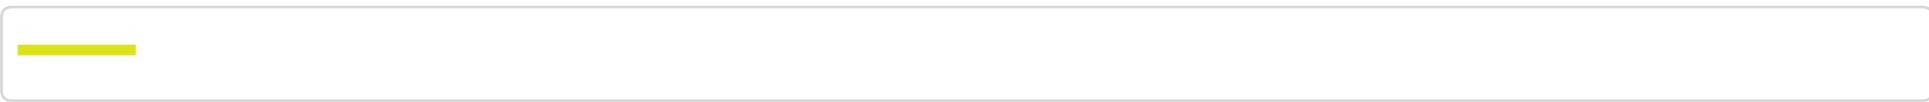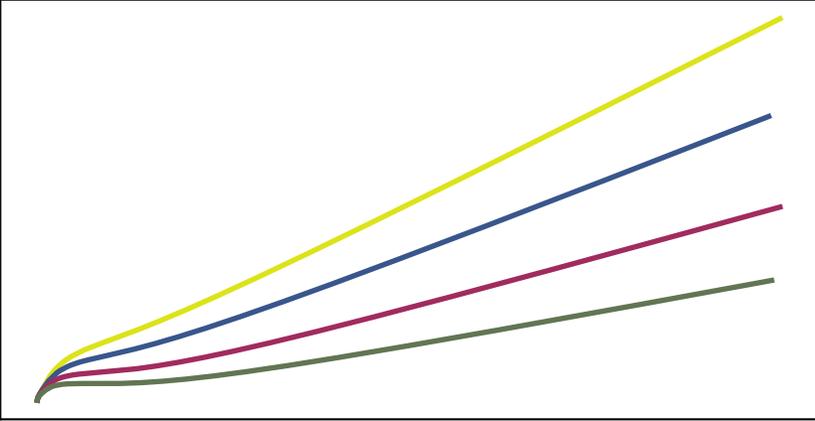

\_\_\_\_\_
