# Supplementary material for: AdaBest: Minimizing Client Drift in Federated Learning via Adaptive Bias Estimation
Source: arXiv:2204.13170 source file (2023-07-24)

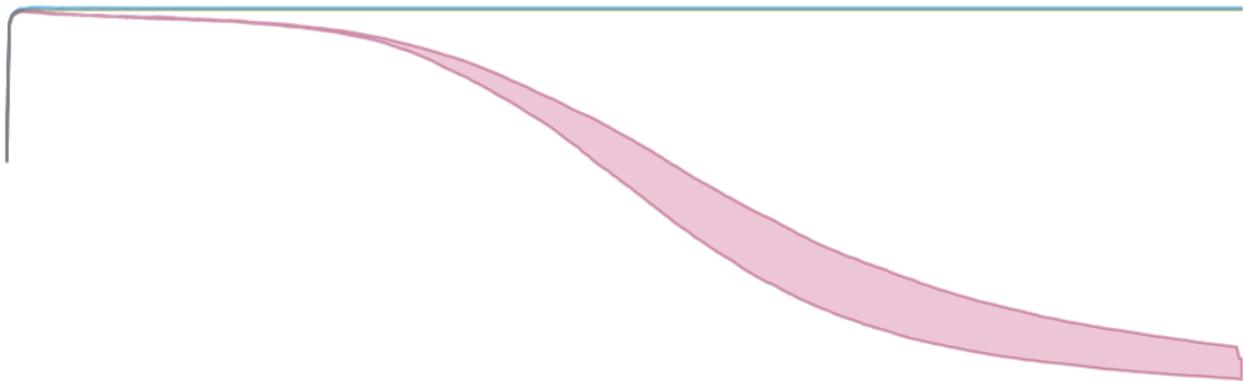









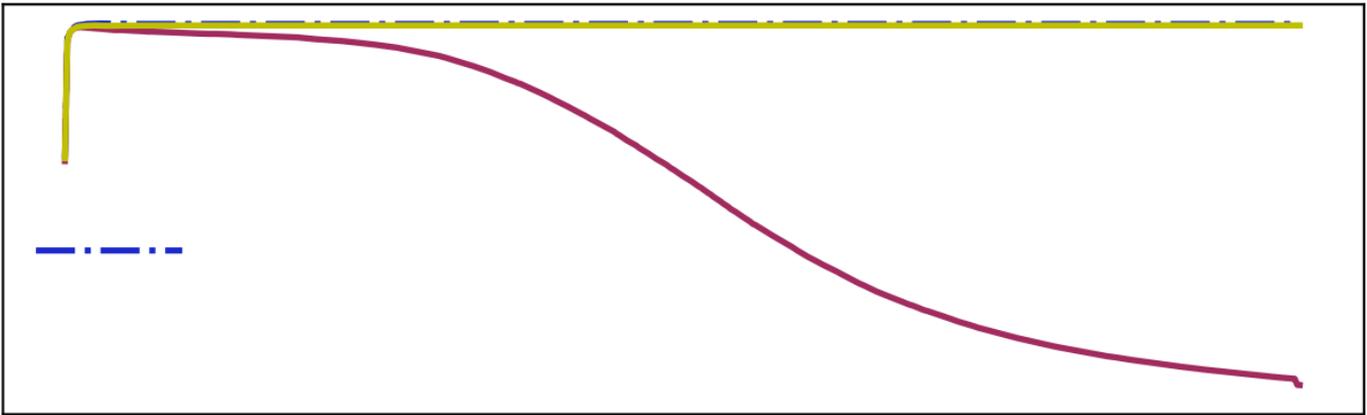

\_\_\_\_\_

\_\_\_\_\_

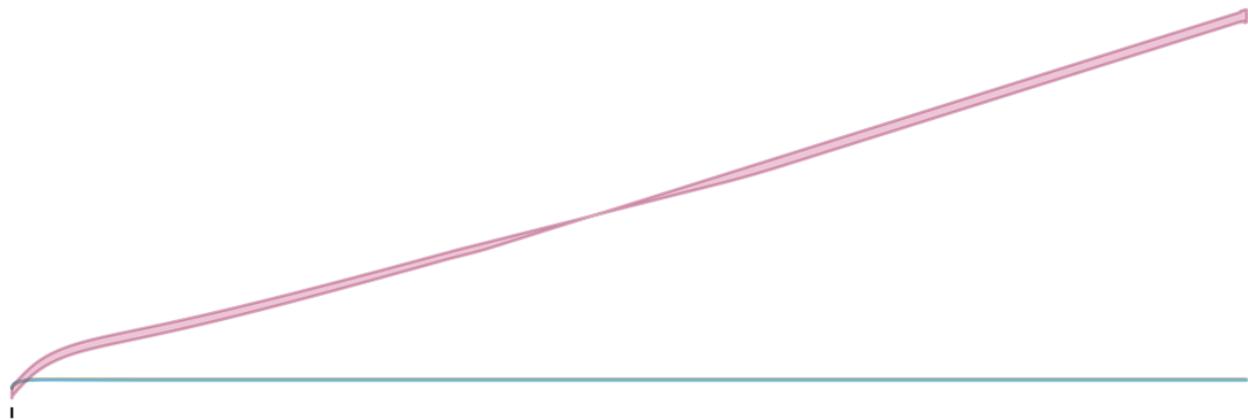























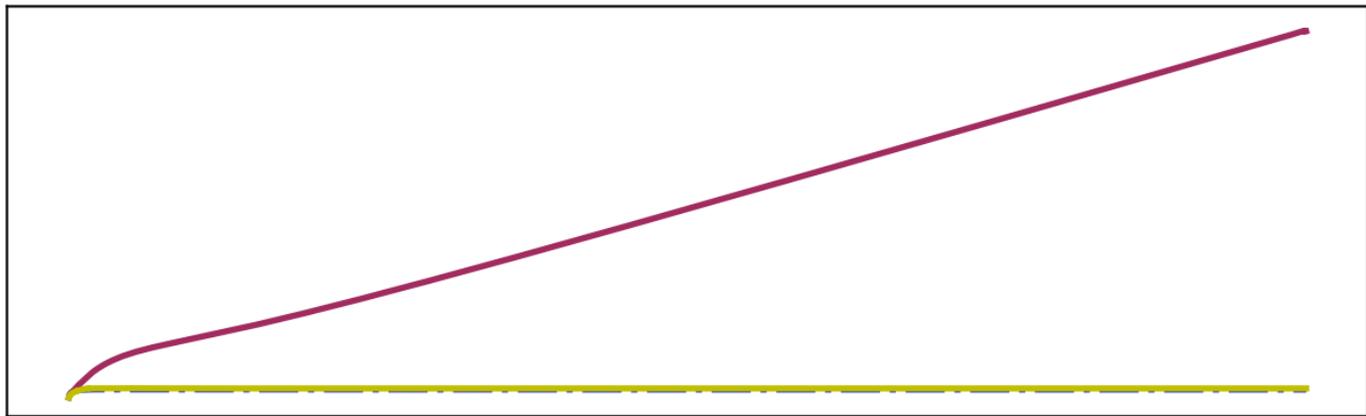

Supplement: Supplementary file 4 [file stability_emnist.pdf]
